# Supplementary material for: Efficient transport controlled by biharmonic frictional driving
Source: arXiv:2409.10285 ancillary file (2024-10-15)
Supplement: Supplementary file 1 [file SupplementalMaterial.pdf]

# Supplemental Material for “Efficient transport controlled by biharmonic frictional driving”

Martin Maza-Cuello and Diego Maza  
*Departamento de Física y Matemática Aplicada, Facultad de Ciencias,  
Universidad de Navarra, E-31080 Pamplona, Spain*  
(Dated: July 5, 2024)

This Supplemental Material includes a technical discussion of the materials and techniques used in the experimental setup and measurements; Supplemental Figures and the description of the Supplemental Videos; and derivations within the NS approximation.

## 1. EXPERIMENTAL SETUP

In the main text (MT), Fig. 1 (a) illustrates a schematic view of the setup used for conducting all experiments. The horizontal tray was connected to a Ling LDS V409 electromechanical shaker to vibrate longitudinally and perpendicularly with respect to gravity. Four lateral high-precision linear bearings (red elements in the figure) constrained its motion longitudinally. A 3-axis accelerometer (blue cube in the figure) monitored the acceleration in the direction of the displacement and its perpendicular directions. The entire setup was mounted on a heavy base to ensure its stability over time. Indeed, in the most extreme explored scenario, the Signal-to-Noise Ratio (SNR) for longitudinal signal acceleration was better than -38 db. Noisy signals with zero mean and standard deviations  $\sigma_y = 0.02 \text{ m s}^{-2}$ ,  $\sigma_z = 0.23 \text{ m s}^{-2}$  in the  $y$  and  $z$  directions respectively were recorded under the same conditions.

A brass cylinder was used as the mass for the results reported in the MT, of diameter 30 mm and height 15 mm, weighting  $m = 80.1 \text{ g}$ . Its bottom surface was accurately machined to leave a knife edge around its periphery and finally polished with 3000-grit sandpaper to minimize contact area and provide better compliance. This design minimizes the contact area and provides robust mechanical stability. The circular geometry exhibits extreme sensitivity to surface heterogeneities, which could potentially induce lateral displacements or rotations in the mass. After the careful polish protocol, no lateral displacement or torsional movements were detected under the range of parameters explored in this study. The other masses tested under the same conditions were cylinders of polymethyl-methacrylate (PMMA) and aluminum. The complete list of specifications is summarized in Table I. All phenomena reported for the brass mass was reproducible with the other cylinders in the same  $\gamma$  range.

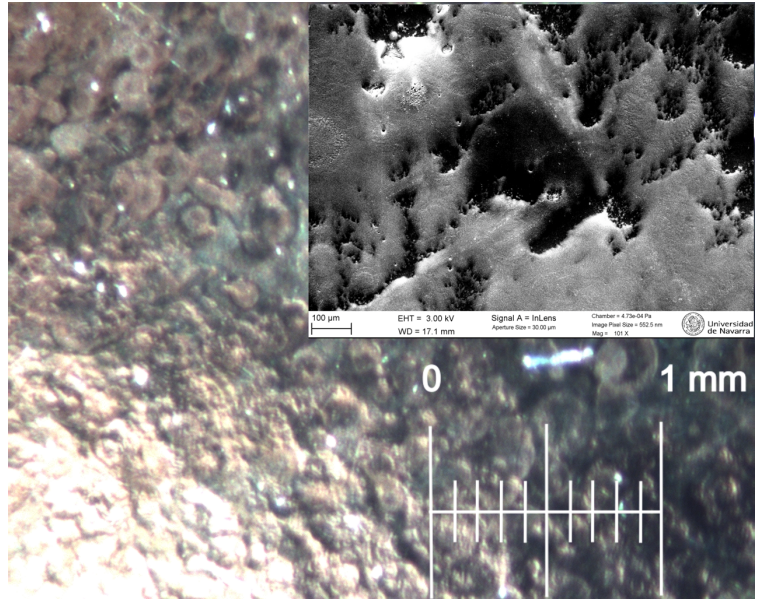

SUP. FIG. 1. Microscopic shadowgraphy of the optical diffuser used as oscillating surface. The inset is a STEM detail of the same surface.

Two different oscillating surfaces were used to test the different masses: (a) an optical quality quartz window (flatness quality  $1\lambda$  per inch @ 633nm) measuring 210 mm in length and 150 mm in width glued to the tray, and

| Type     | Diameter<br>(mm) | Mass<br>(g) | Ring width<br>(mm) |
|----------|------------------|-------------|--------------------|
| Brass    | 30.0             | 80.1        | 0.15               |
| PMMA     | 39.2             | 17.93       | 0.75               |
| Aluminum | 28.0             | 12.26       | 0.20               |

TABLE I. Properties of the masses used in the experiments.

(b) a 120-grit ground optical glass diffuser (Edmund Optics) of the same dimensions. The optical quality of the glass guarantees global surface flatness, whereas the “lunar landscape” of the microscopic diffuser structure (see Sup. Fig. 1) guarantees the statistical homogeneity of surface properties. Each base was leveled using a high-precision spirit level with a resolution of 0.02 mm per meter. Before each experimental run, the base and mass surfaces were cleaned with acetone and isopropyl alcohol. Notably, observed dynamics remained unaffected even when the surfaces were intentionally contaminated.

The dynamics of the base and mass were characterized using two synchronized high-speed cameras (Photron MiniUX). The image acquisition system was synchronized with accelerometer output signals using a data logger (NI USB-X-6361). Macro lenses were employed to achieve a spatial resolution better than 15  $\mu\text{m}$ . This combination allows us to ensure that the shaker performs as expected under the action of the applied signal. These signals were generated by Function/Arbitrary Waveform Generator, Agilent 33521A. Despite the high quality of its output signal, a careful calibration protocol must be implemented to reach the desired shaker vibrations due to its low-frequency nonlinear response. Therefore, the amplitude and phase difference of the superposed harmonic signals delivered by the waveform generator was tuned meticulously (not precisely with its hypothetical, theoretical values) to reach the theoretically expected base acceleration. Microscopic movements of the mass were analyzed until frame rates as large as 200,000 fps to guarantee that no essential feature for describing the overall macroscopic drift was neglected under current experimental conditions. All data reported in the MT was recorded at 5,000 fps. Supplemental Videos are recorded at a standard frame rate and show the dynamics in real time.

## 2. SUPPLEMENTAL FIGURES

Supplemental Figure 2 shows the velocity of the walker  $v(t)$  during one period  $T = 50\text{ ms}$ , with data obtained at 200,000 fps. The inset shows a detail of the transition between slip steps, which takes place over a time interval  $\tau \sim 2\text{ ms} \ll T$ . Supplemental Figure 3 shows long-term trajectories  $x(t)$  of the brass walker, complementing Fig. 2(a) on the MT. The trajectories are stable over time intervals much longer than the oscillation period  $T$  of the base for all cases analyzed. To obtain the averaged data of Fig. 2(a) in the MT, the trajectories are cut into windows of duration  $T$ , and windows are averaged after subtracting their corresponding initial positions. Supplemental Figure 4 compares the drift velocity  $v_D$  as a function of  $\gamma$  for different materials and for two values of the phase,  $\varphi = 0$  and  $\pi/2$ .  $v_D$  is found to grow linearly with  $\gamma$  in the  $\varphi = 0$  case [panel (a)] and to saturate for  $\varphi = \pi/2$  [panel (b)] for all three materials. Supplemental Figure 5 shows the velocity  $v(t)$  of the different walkers when the quartz surface is used, for biharmonic signals with  $\gamma/g = 2$  and indicated values of  $\varphi$ . No qualitative difference is observed among the materials. Comparing these panels with Figs. 2(c) and 2(d) of the MT, it is seen that the dynamics are overall unaffected by the change of substrate.

## 3. SUPPLEMENTAL VIDEOS

Supplemental Video 1 shows the drift of the brass mass in real time for the biharmonic signal [see Eq. (1) in the MT] with  $\omega = 125.66\text{ 1/s}$ ,  $\rho = 1/2$ ,  $\gamma/g = 0.68$  and  $\varphi = \pi/2$ . Physical properties of the mass are listed in Table I. Supplemental Video 2 exemplifies the surprising effect that, for certain oscillations, an inversion of the transport direction may occur when increasing  $\gamma$ . In the video, the target on the bottom is glued to the base as a reference of the amplitude of the base oscillation. This amplitude is increased from zero during the first half of the video and then decreased again to zero. Supplemental Video 3 shows the simultaneous motion of two objects made out of brass: one the aforementioned 80.1 g walker and the other a solid cylinder of mass 2.5 kg. Both have the same drift velocity.

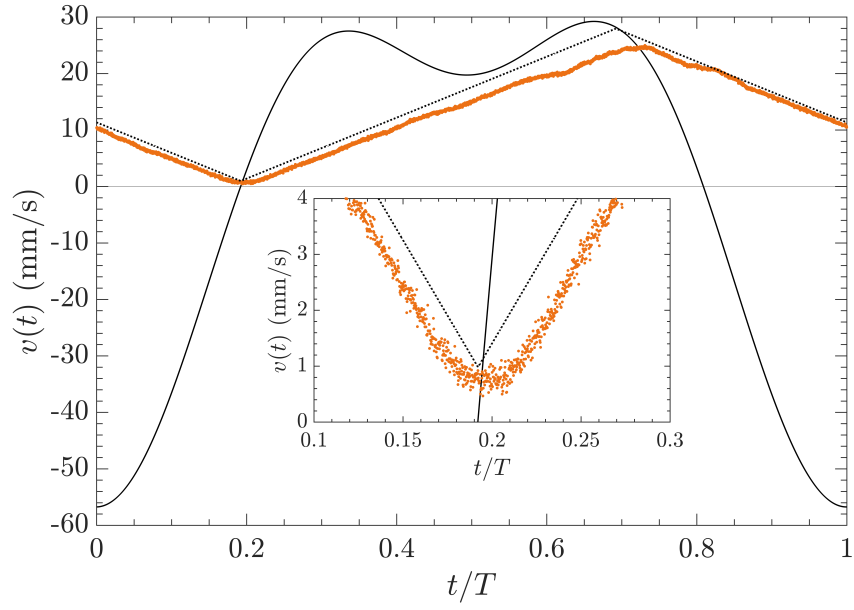

SUP. FIG. 2. Averaged velocity of the brass walker  $v(t)$  (orange points) for  $\varphi = 0$  and  $\gamma = g$ , from data obtained at 200,000 fps. Solid curve is the base velocity  $v_B(t)$ . Dotted curve is the expected velocity cycle computed from the NS approximation (see MT for details). Inset: detail of the transition between slip steps.

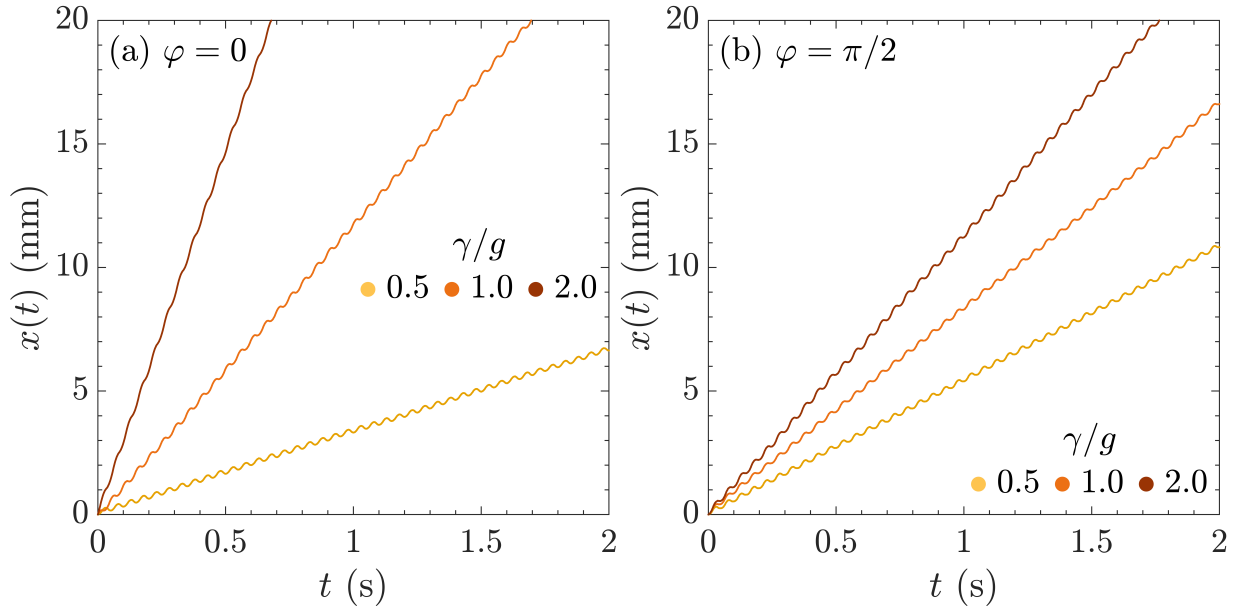

SUP. FIG. 3. Comparison of long-term trajectories  $x(t)$  of the brass walker for (a)  $\varphi = 0$  and (b)  $\varphi = \pi/2$ .

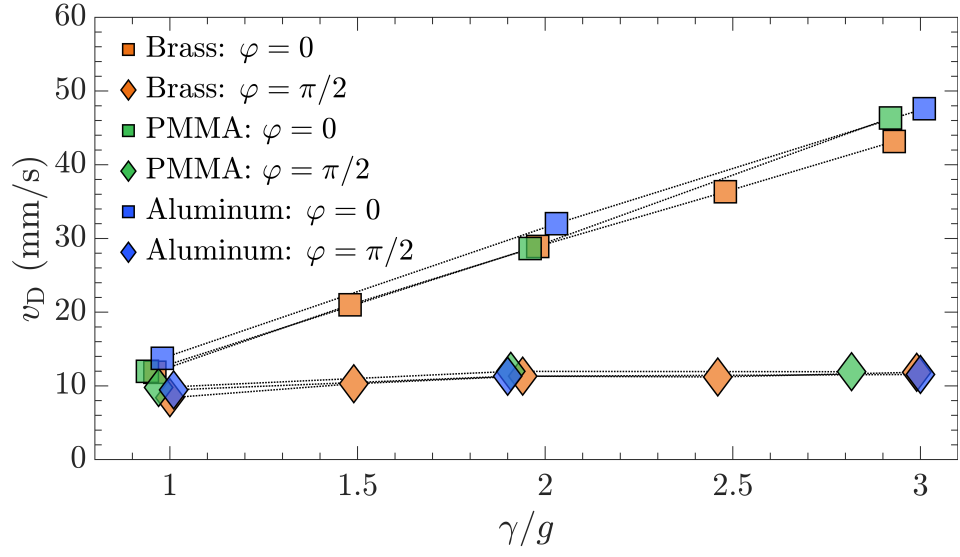

SUP. FIG. 4. Comparison of drift velocity  $v_D$  as a function of  $\gamma$  for different materials. Lines are guides to the eye.

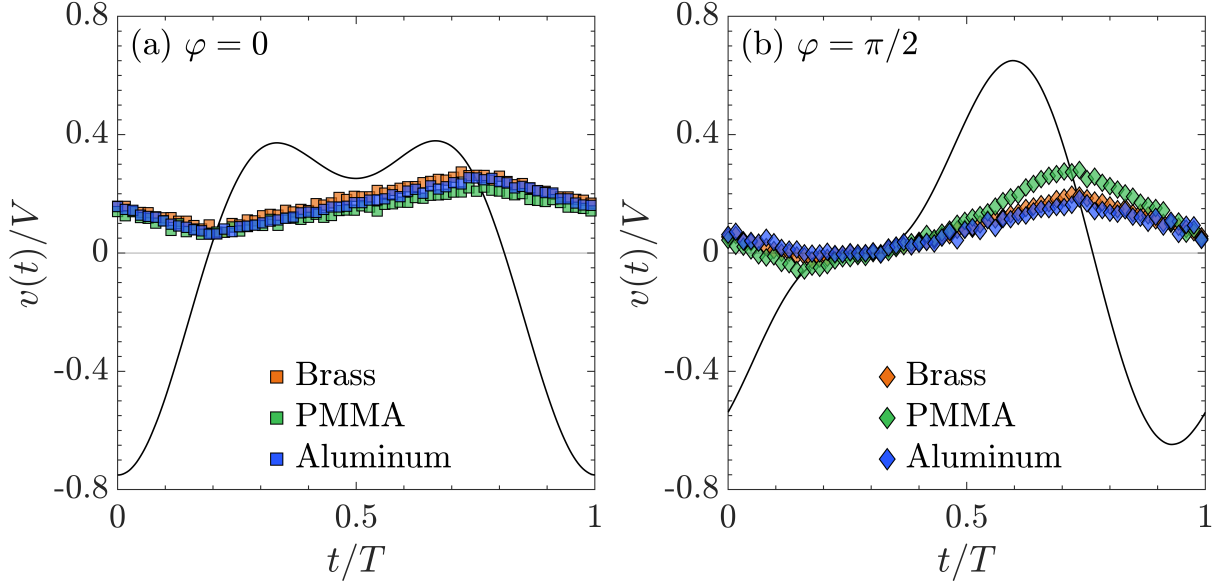

SUP. FIG. 5. Comparison of walker velocity  $v(t)$  for walkers of different materials over an optical quality quartz window. (a)  $\varphi = 0$ . (b)  $\varphi = \pi/2$ . In both panels,  $\gamma = 2g$ .

#### 4. NS APPROXIMATION FOR A MULTIHARMONIC SIGNAL

Let the base velocity  $v_B(t)$  be a multiharmonic composition of odd and even multiples of a fundamental frequency  $\omega$  (fundamental period  $T = 2\pi/\omega$ ),

$$v_B(t) = -V \left\{ \sum_{q=1}^n a_q \cos([2q-1]\omega t + \alpha_q) + \sum_{p=1}^m b_p \cos(2p\omega t + \beta_p) \right\}, \quad (\text{SM1})$$

with  $V = \sqrt{2}V_{\text{RMS}}$  the peak velocity of the family and a measure of the input energy,  $\alpha_q$  and  $\beta_p$  phases, and  $a_q$  and  $b_p$  non-negative dimensionless weights ( $a_1 > 0$ ), normalized such that  $\sum a_q^2 + \sum b_p^2 = 1$ .

For large input energy, corresponding to a large  $V$  in Eq. (SM1), we assume that the walker is always slipping, resulting in a piece-wise linear evolution of the walker's velocity  $v(t)$ . Clearly  $v(t)$  may have several slip steps during a period. Requiring  $v(t)$  to be cyclic with period  $T$ , the linear nature of the steps imply that the expected macroscopic drift  $v_D$  would be the same if they are rearranged into a single step in each direction, each one lasting  $T/2$ . This rearrangement allows to directly apply the procedure discussed in the MT for the biharmonic signal.

To find the drift velocity according to the NS approximation, first one should find the time  $t_0$  satisfying Eq. (5) of the MT,

$$v_B(t_0 + T/2) - v_B(t_0) = \mu g \frac{T}{2}. \quad (\text{SM2})$$

Using Eq. (SM1), Eq. (SM2) reads

$$\sum_{q=1}^n a_q \cos([2q-1]\omega t_0 + \alpha_q) = \frac{\mu g T}{4V}. \quad (\text{SM3})$$

Note that only odd harmonics appear in this equation.

Assuming  $V$  is large enough so that a solution can be found, by using Eq. (6) of the MT

$$v_D^{\text{NS}} = \frac{v_B(t_0) + v_B(t_0 + T/2)}{2}, \quad (\text{SM4})$$

the resulting drift velocity is

$$v_D^{\text{NS}} = V \sum_{p=1}^m b_p \cos(2p\omega t_0 + \beta_p). \quad (\text{SM5})$$

Therefore, the magnitude of the drift is controlled solely by the even harmonics, and  $v_D^{\text{NS}}$  may grow proportionally with  $V$  unless  $v_B(t)$  only contains odd harmonics, in which case  $v_D^{\text{NS}} = 0$  always.

## 5. FRICTION-INDEPENDENT EFFICIENCY BOUND

In the limit of very large base acceleration  $\gamma/g \gg \pi\mu$ , the optimal phase given by Eq. (8) of the MT shifts towards  $\Theta \rightarrow 0$  and the efficiency depends on the phase as

$$\eta^{\text{NS}}|_{\gamma/g \gg \pi\mu} = \sqrt{\frac{2}{5}} \cos(\varphi). \quad (\text{SM6})$$

Surprisingly, this limiting behavior of the transport efficiency is independent of friction. This is a general feature of the efficiency for any periodic base oscillation in this limit under the friction model given by Eq. (2) of the MT. To see why, notice that writing this model in dimensionless variables  $\tilde{t} = \omega t$ ,  $\tilde{v} = v/V_{\text{RMS}}$ ,

$$\dot{\tilde{v}}(\tilde{t}) = -\frac{\mu g}{\omega V_{\text{RMS}}} \text{sgn} \{ \tilde{v}_R(\tilde{t}) \}, \quad (1)$$

predicts a constant velocity  $\tilde{v}$  as  $V_{\text{RMS}} \rightarrow \infty$ . This value is identical with the limiting value of the (dimensionless) drift velocity  $\tilde{v}_D^\infty$  and thus an upper bound for  $\eta$ . The constant  $\tilde{v}_D^\infty$  is *not* arbitrary: it is the only value for which the time intervals between the solutions  $\{t_i\}$  of  $\tilde{v}_B(t_i) = \tilde{v}_D^\infty$  make  $\tilde{v}_R$  be positive (or negative) during half a period, hence producing the required cycle satisfying Eq. (3) of the MT. Since the biharmonic signal leads to only two steps, it is simple to check that  $\tilde{v}_D^\infty(\varphi = \pi/2) = 0$  and  $\tilde{v}_D^\infty(\varphi = 0) = \sqrt{2/5}$ , exactly as predicted by Eq. (SM6).
